# Supplementary material for: Predicting Drug Responses by Propagating Interactions through Text-Enhanced Drug-Gene Networks
Source: arXiv:1906.08089 source file (2019-06-19)
Supplement: Supplementary file 1 [file 5_appendix.tex]

\appendix
\begin{appendices}
\section{Datasets}

\begin{figure}[H]
    \vspace{-1cm}
    \centering
    \caption{Number of Categorical Interactions in DGIdb}
    \includegraphics[width=\linewidth]{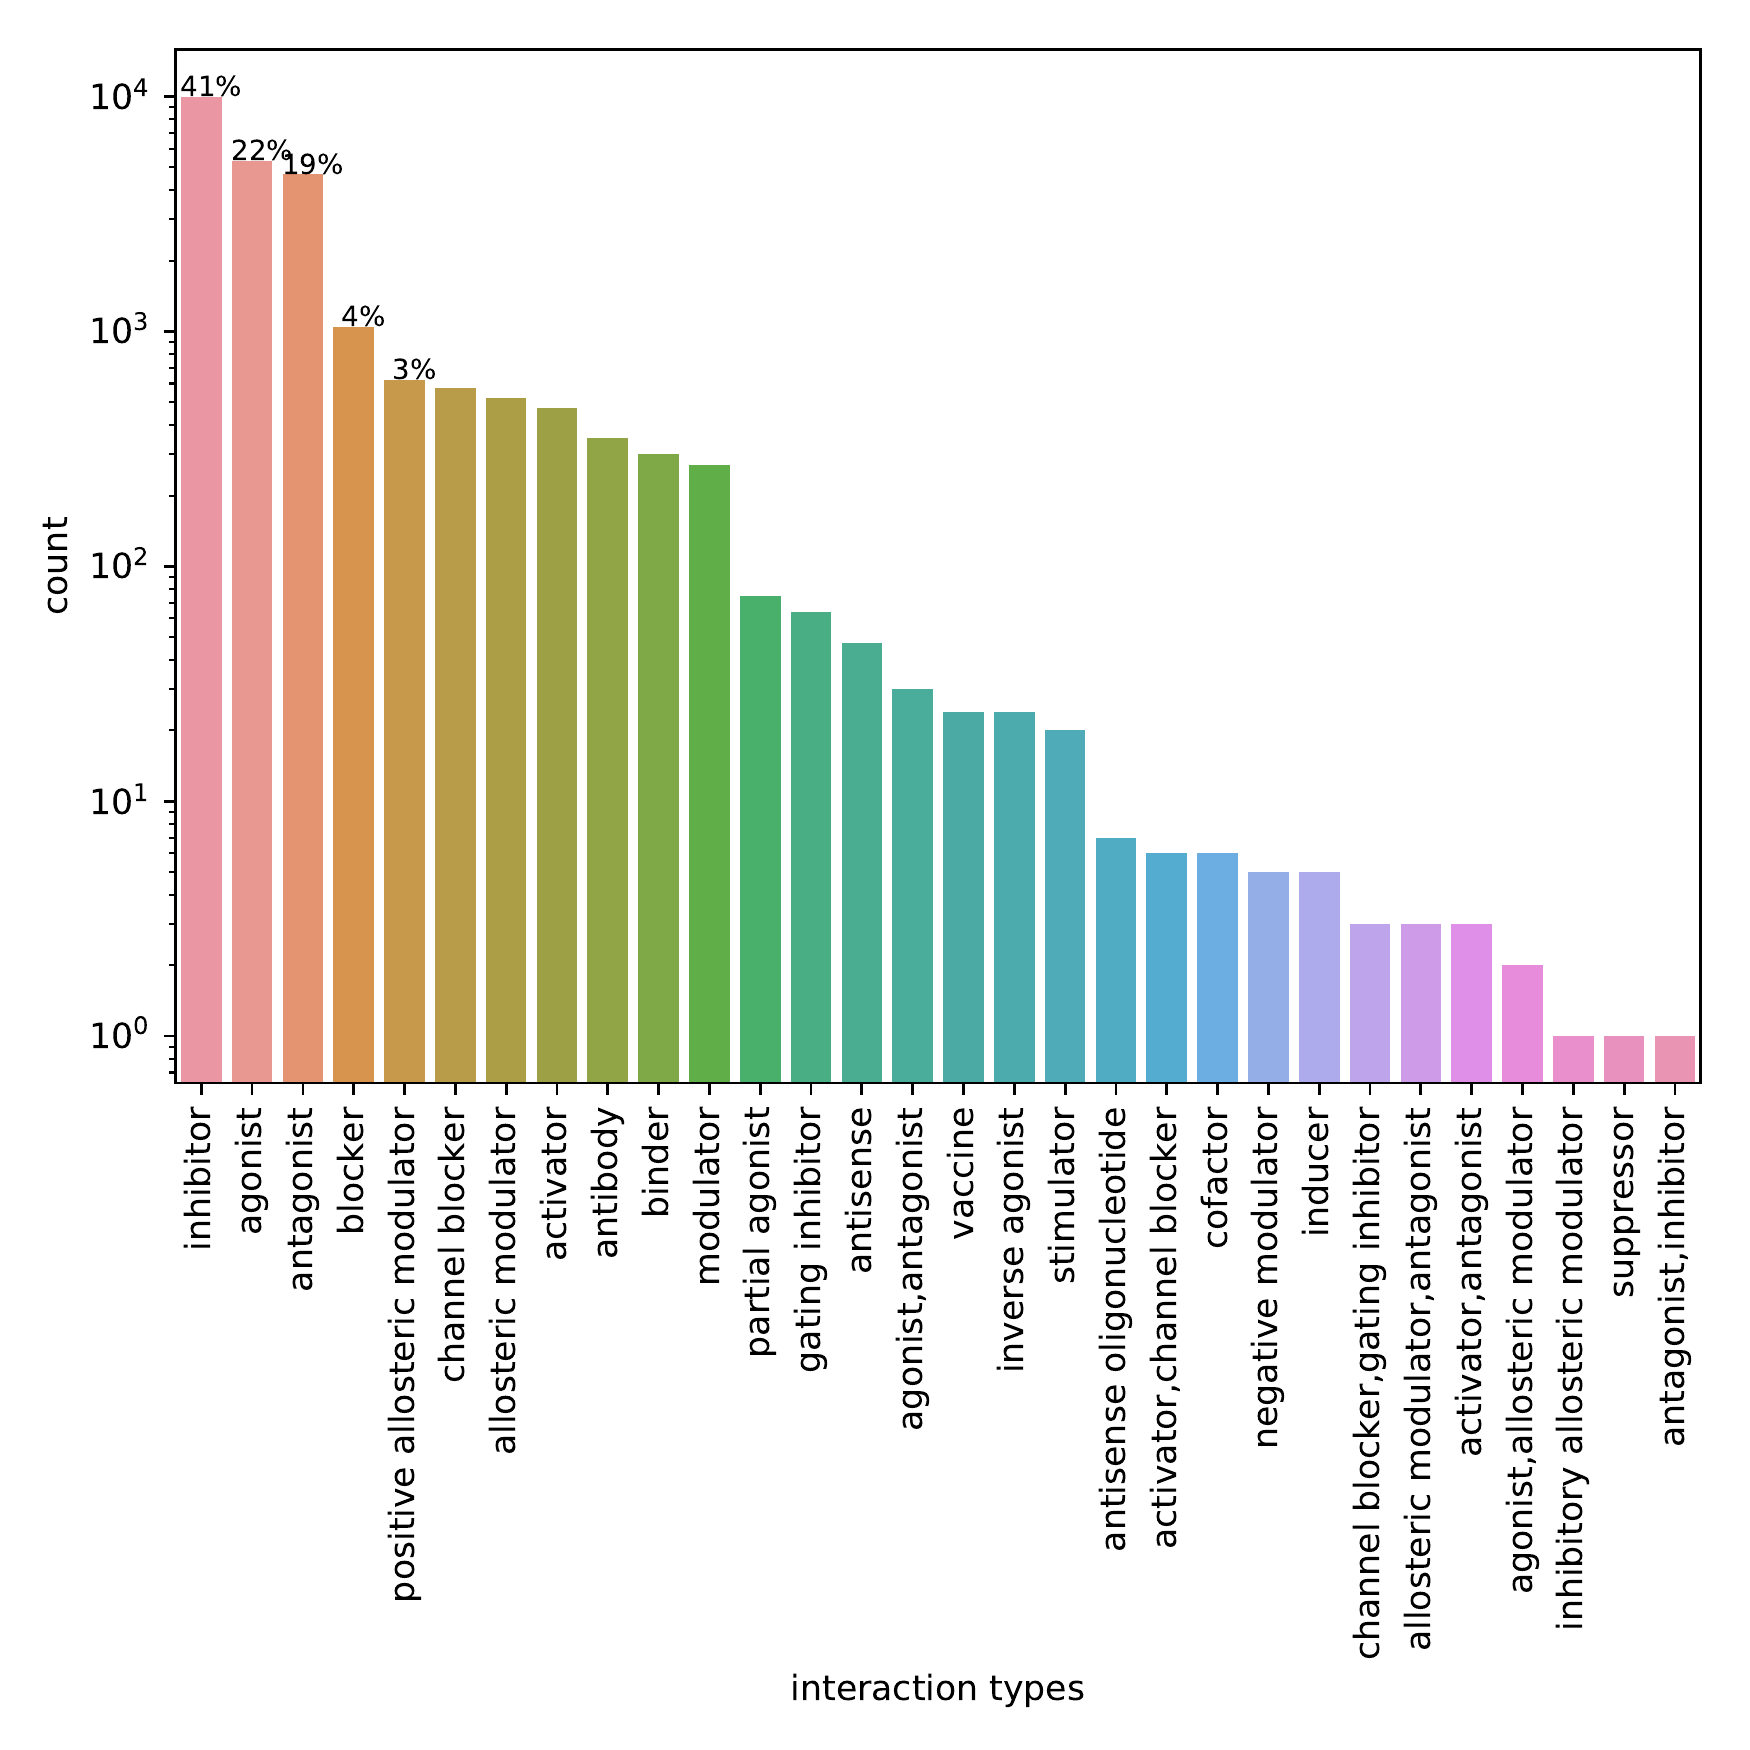}
    \label{fig:count_plot}
\end{figure}

\begin{figure}[H]
\vspace{-1cm}
    \centering
    \caption{Number of Meta-Pattern Pairs}
    \includegraphics[width=\linewidth]{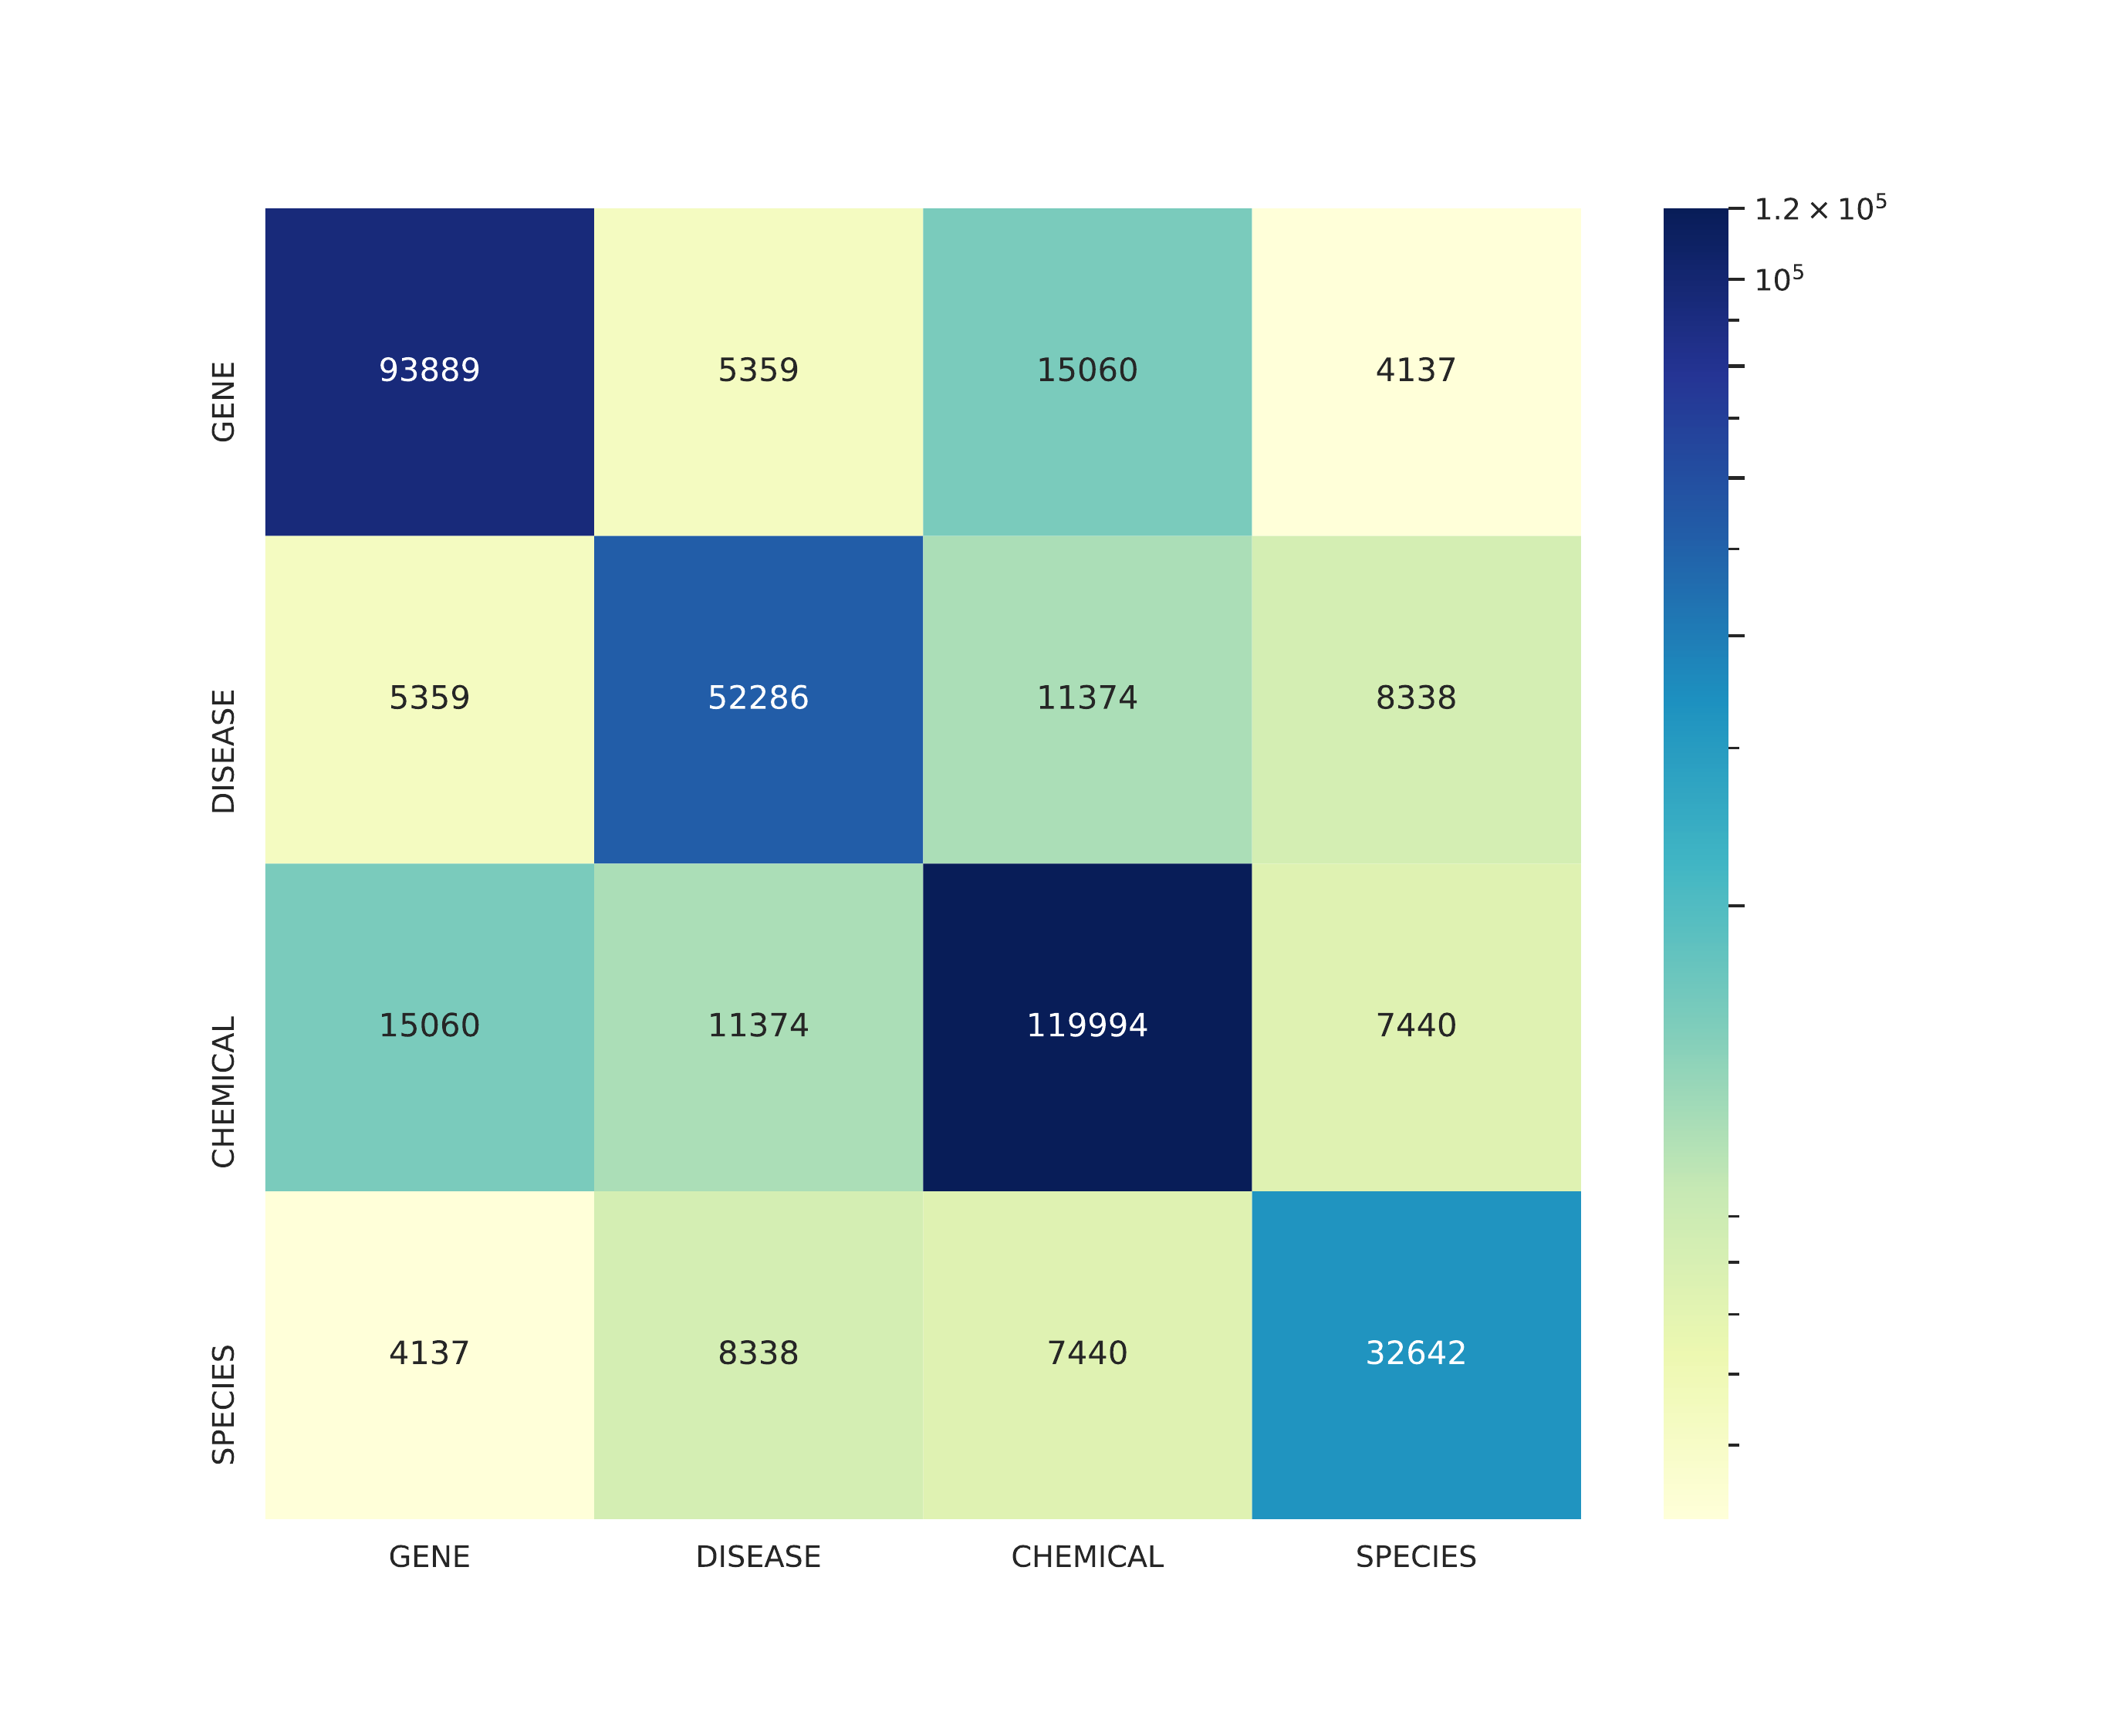}
    \label{fig:pairs}
\end{figure}

\end{appendices}
